# Supplementary material for: Approximation and Hardness for Token Swapping
Source: arXiv:1602.05150 source file (2016-08-02)
Supplement: Supplementary file 1 [file Appendix.tex]

%\section*{Appendix}
%For the proof of Theorem~\ref{thm:main}, it might be convenient for the reader to play around with the possible moves, so we provide here a printable version that can be printed and cut out at ones pleasure.
%From personal experience, we further recommend to glue the black 
%tokens to some cardboard and cut them out thereafter.

%\newpage\null\thispagestyle{empty}\newpage
%\newpage\null\thispagestyle{empty}\newpage

\centering
\thispagestyle{empty}
\begin{figure}%
\includegraphics[angle=90, width = 1.1\textwidth]{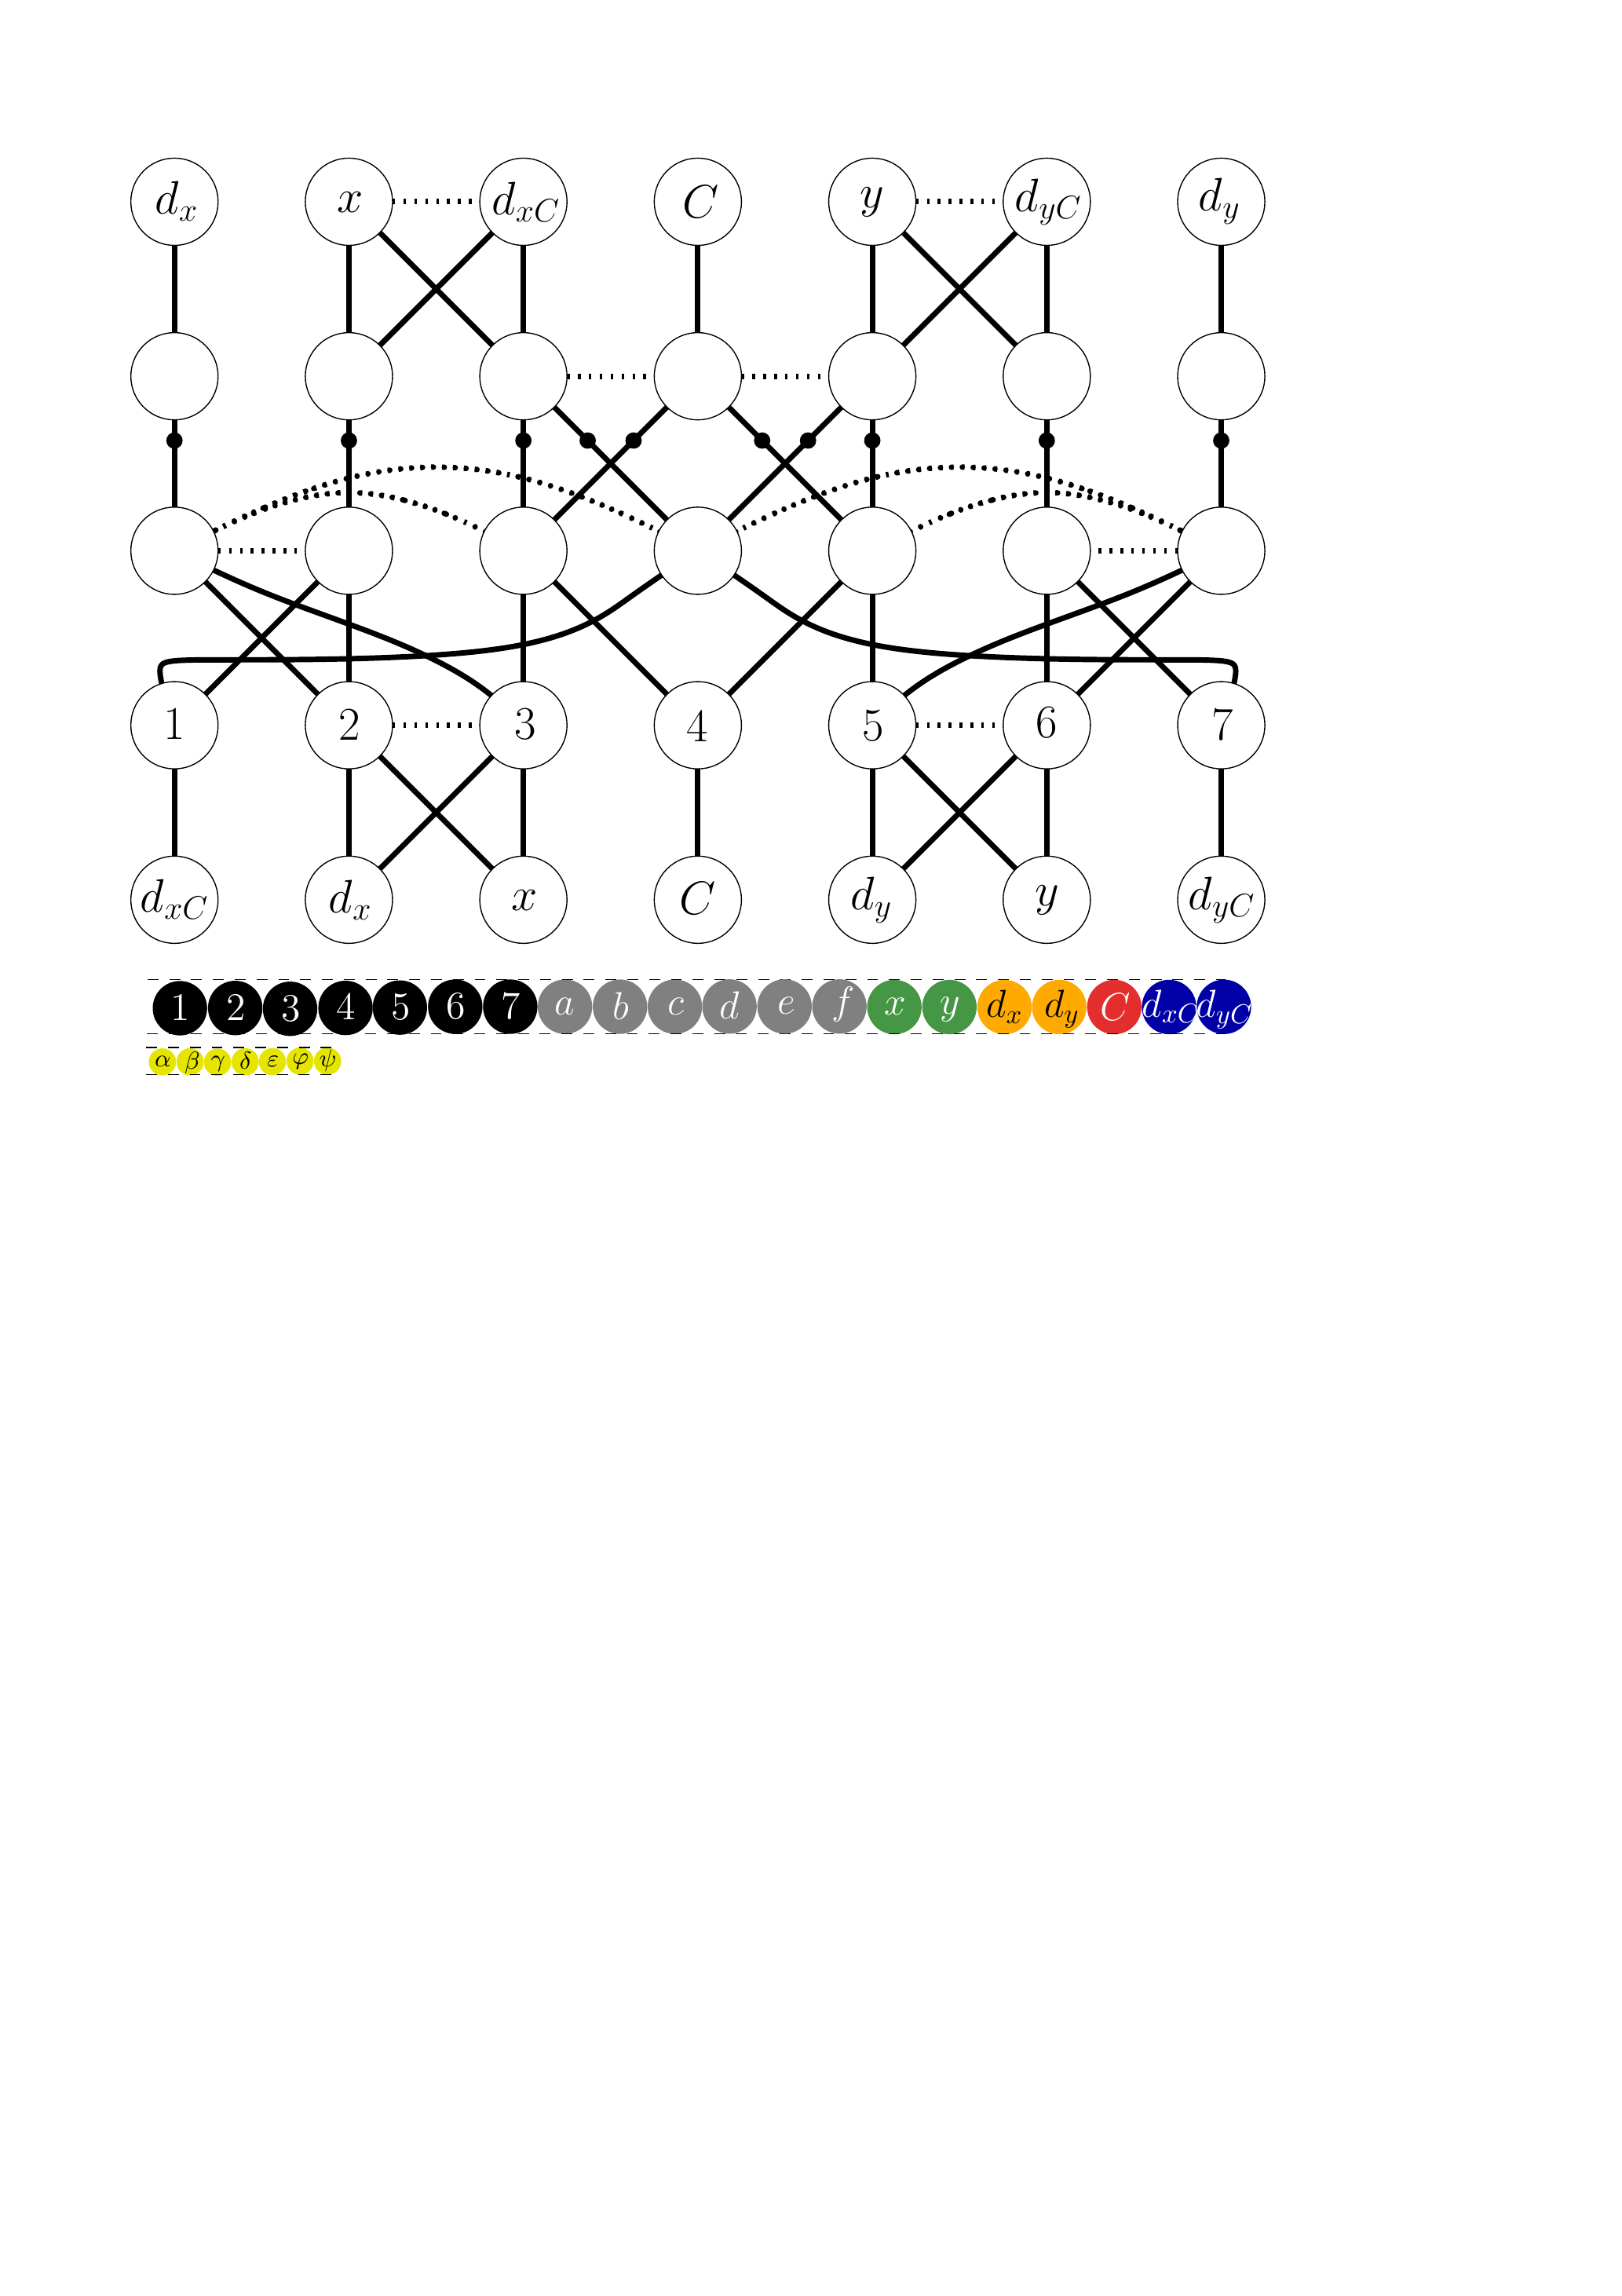}
\vspace{1cm}
\caption{The gadget to play around and test yourself.
The tokens $1-7$, $a-f$ and $\alpha - \psi$ can be used everywhere.
Every vertex in the top row, wants to go to
the vertex on the bottom row with the same label.
The tokens on the vertices indicated with a small black dot
want to stay where they are. 
All other vertics want to move to the vertex exactly one layer up.
(Except that the layer of small black dots is skipped).
(The drawing is rotated by 90 degree.)}%
\label{}%
\end{figure}
